# Supplementary material for: Pseudo-Stereo for Monocular 3D Object Detection in Autonomous Driving
Source: arXiv:2203.02112 source file (2022-03-04)
Supplement: Supplementary file 1 [file supp.pdf]

# Pseudo-Stereo for Monocular 3D Object Detection in Autonomous Driving

## Supplementary Material

Yi-Nan Chen<sup>1</sup> Hang Dai<sup>2\*</sup> Yong Ding<sup>1\*</sup>

<sup>1</sup>School of Micro-Nano Electronics, Zhejiang University

<sup>2</sup>Mohamed bin Zayed University of Artificial Intelligence, Abu Dhabi, UAE

\*Corresponding authors{hang.dai@mbzuai.ac.ae, dingy@vlsi.zju.edu.cn}.

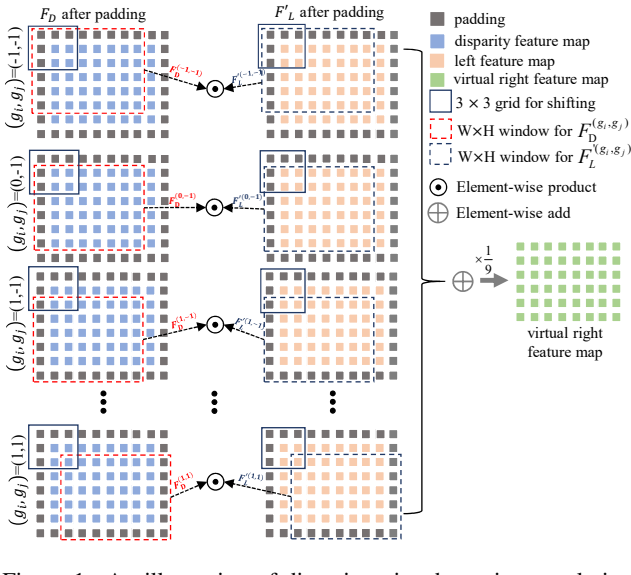

Figure 1. An illustration of disparity-wise dynamic convolution with grid shifting. The top left corner point of  $W \times H$  window (blue and red dot windows for disparity feature map and left feature map, respectively) shifts within the  $3 \times 3$  grid (blue box). The outcome (virtual right feature map) of the overall operation with 9 times  $W \times H$  window shifting in  $3 \times 3$  grid is the same as that of the overall operation with  $W \times H$  times  $3 \times 3$  sliding window to cover the whole feature map.

### 1. Disparity-wise Dynamic Convolution with Grid Shifting

The process of disparity-wise dynamic convolution with grid shifting can be formulated as:

$$\hat{F}'_R = \frac{1}{3 \times 3} \sum_{g_i, g_j} F'_L^{(g_i, g_j)} \odot F_D^{(g_i, g_j)} \quad (1)$$

where  $\hat{F}'_R$  is the generated virtual right feature map,  $F'_L$  indicates the left feature map and  $F_D$  is the disparity feature map. The  $(g_i, g_j)$  indicates the shifting direction and step size within the  $3 \times 3$  grid  $\{(g_i, g_j)\}$ , where  $g \in \{-1, 0, 1\}$ .

Also, the Eqn. 1 can be expanded as follows:

$$\begin{aligned} \hat{F}'_R = & \frac{1}{3 \times 3} (F'_L^{(-1, -1)} \odot F_D^{(-1, -1)} \\ & + F'_L^{(-1, 0)} \odot F_D^{(-1, 0)} + F'_L^{(-1, 1)} \odot F_D^{(-1, 1)} \\ & + F'_L^{(0, -1)} \odot F_D^{(0, -1)} + F'_L^{(0, 0)} \odot F_D^{(0, 0)} \\ & + F'_L^{(0, 1)} \odot F_D^{(0, 1)} + F'_L^{(1, -1)} \odot F_D^{(1, -1)} \\ & + F'_L^{(1, 0)} \odot F_D^{(1, 0)} + F'_L^{(1, 1)} \odot F_D^{(1, 1)}) \end{aligned} \quad (2)$$

We illustrate the above process in Figure 1. The top left corner point of  $W \times H$  window (blue and red dot windows for disparity feature map and left feature map, respectively) shifts within the  $3 \times 3$  grid (blue box). The outcome (virtual right feature map) of the overall operation with 9 times  $W \times H$  window shifting in  $3 \times 3$  grid is the same as that of the overall operation with  $W \times H$  times  $3 \times 3$  sliding window to cover the whole feature map.

### 2. Right Feature Re-projection in Feature-clone

In the main paper, we follow LIGA-stereo [3] to concatenate the left features  $F_L$  and the re-projected right features  $F_{R \rightarrow L}$  at all candidate depth levels for building the stereo volume  $V_{st}$  as follows:

$$V_{st}(u, v, w) = \text{concat}[F_L(u, v), F_{R \rightarrow L}(u, v)] \quad (3)$$

$$F_{R \rightarrow L}(u, v) = F_R(u - \frac{f \cdot b}{d(w) \cdot S}, v) \quad (4)$$

$$d(w) = w \cdot v_d + z_{min} \quad (5)$$

where  $(u, v)$  are the pixel coordinates,  $w \in [0, 1, \dots]$  indicates the depth index,  $S$  is the stride of the feature map,  $v_d$  is the depth interval,  $z_{min}$  indicates the minimal depth value,  $f$  is the camera focal length, and  $b$  represents the baseline of the stereo camera pair. In feature-clone virtual right view generation method, we duplicate the left features  $F_L$  as the right features  $\hat{F}_R$  and concatenate the left features  $F_L$  and re-projected right features  $F_{R \rightarrow L}$  as described in Eqn. 3.

| Methods                    | $AP_{3D}/AP_{BEV}$   |                      |                      |
|----------------------------|----------------------|----------------------|----------------------|
|                            | Easy                 | Moderate             | Hard                 |
| Ours-fcd w/ re-projection  | <b>28.46 / 37.66</b> | <b>19.15 / 25.78</b> | <b>16.56 / 22.47</b> |
| Ours-fcd w/o re-projection | 22.36 / 31.49        | 16.19 / 22.68        | 14.19 / 20.48        |

Table 1. Performance for *Car* on KITTI *val* set at IOU threshold 0.7. Compare the performance with and without re-projection. We report the results in  $AP|_{R40}$ .

To show the effectiveness of the right feature re-projection, we conduct an experiment using the the concatenation of the left features  $F_L$  and the virtual right features  $\hat{F}_R$  without re-projection as:

$$V_{st}^*(u, v, w) = \text{concat}[F_L(u, v), \hat{F}_R(u, v)] \quad (6)$$

As shown in Table. 1, without re-projection, the performance of the proposed framework decreases significantly in  $AP_{3D}$  by (-6.1%, -2.96%, -2.37%) and  $AP_{BEV}$  by (-6.17%, -3.1%, -1.99%). This implies that the re-projection of right feature is effective in constructing the stereo volume for monocular 3D detection.

| Exp. | Methods       | $L_{depth}$ | $L_{kd}$ | $AP_{3D}/AP_{BEV}$   |                      |                      |
|------|---------------|-------------|----------|----------------------|----------------------|----------------------|
|      |               |             |          | Easy                 | Moderate             | Hard                 |
| 1    | Image-level   | ✓           | ✓        | 31.43 / 41.82        | 21.53 / 29.00        | 18.47 / 25.21        |
| 2    | Image-level   | ✓           | ✓        | <b>31.81 / 42.87</b> | <b>22.36 / 30.16</b> | <b>19.33 / 26.38</b> |
| 3    | Image-level   | ✓           | ✓        | 29.10 / 39.61        | 20.12 / 27.60        | 17.07 / 23.16        |
| 4    | Image-level   | ✓           | ✓        | 28.89 / 40.17        | 20.79 / 29.45        | 17.81 / 25.14        |
| 5    | Feature-level | ✓           | ✓        | <b>35.18 / 45.50</b> | <b>24.15 / 32.03</b> | <b>20.35 / 27.57</b> |
| 6    | Feature-level | ✓           | ✓        | 22.04 / 31.10        | 16.18 / 22.55        | 14.31 / 20.56        |
| 7    | Feature-level | ✓           | ✓        | 32.48 / 43.62        | 22.38 / 30.78        | 19.23 / 26.94        |
| 8    | Feature-level | ✓           | ✓        | 19.37 / 29.44        | 14.10 / 21.26        | 12.55 / 19.22        |
| 9    | Feature-clone | ✓           | ✓        | <b>28.46 / 37.66</b> | <b>19.15 / 25.78</b> | <b>16.56 / 22.47</b> |
| 10   | Feature-clone | ✓           | ✓        | 24.33 / 32.99        | 17.09 / 23.77        | 14.61 / 20.81        |
| 11   | Feature-clone | ✓           | ✓        | 24.20 / 33.69        | 17.02 / 23.85        | 14.73 / 21.26        |
| 12   | Feature-clone | ✓           | ✓        | 19.69 / 28.96        | 14.56 / 21.32        | 12.94 / 19.04        |

Table 2. Ablation studies of three proposed Pseudo-Stereo variants,  $L_{depth}$  and  $L_{kd}$  at IOU threshold 0.7. Exp. is the experiment tag. We report the results in  $AP|_{R40}$ .

### 3. The Effect of Knowledge Distillation

Although LIGA-stereo has studied the effect of knowledge distillation in [3], we conduct an extra study of knowledge distillation for the proposed Pseudo-Stereo frameworks in supplementary material as shown in Table. 2. The proposed frameworks without the knowledge distillation still achieve decent performance on KITTI *val* set. As discussed and analyzed in the main paper, the depth loss is not effective for image-level generation. Knowledge distillation improves the detection performance, which is consistent with the study in LIGA-stereo [3]. This lies in the fact that knowledge distillation transfers the structural detection knowledge from LiDAR-based 3D detectors. Note that we focus on the analysis of depth-aware feature learning in the main paper and discuss the knowledge distillation that is

| Methods                 | $L_{disp}$ | $AP_{3D}/AP_{BEV}$          |                             |                             |
|-------------------------|------------|-----------------------------|-----------------------------|-----------------------------|
|                         |            | Easy                        | Moderate                    | Hard                        |
| Pseudo-LiDAR [8]        | –          | – / 28.20                   | – / 18.50                   | – / 16.40                   |
| AM3D [6]                | –          | – / <u>32.23</u>            | – / 21.09                   | – / 17.26                   |
| DDMP-3D [7]             | –          | <u>28.12</u> / 31.14        | <u>20.39</u> / <u>23.12</u> | <b>16.34</b> / <u>19.45</u> |
| M3D-RPN [1]             | –          | 14.53 / 20.27               | 11.07 / 17.06               | 8.65 / 15.21                |
| D4LCN [2]               | –          | 22.32 / 26.97               | 16.20 / 21.71               | 12.30 / 18.22               |
| YOLOMono3D [5]          | –          | 21.66 / –                   | 14.20 / –                   | 11.07 / –                   |
| Ours + YOLOStereo3D [5] | ✓          | <b>33.74</b> / <b>44.95</b> | <b>21.56</b> / <b>28.04</b> | <u>15.58</u> / <b>21.87</b> |
| Ours + YOLOStereo3D [5] | ✓          | 17.79 / 28.01               | 11.20 / 17.63               | 8.81 / 13.55                |

Table 3. Performance for *Car* on KITTI *val* set at IOU threshold 0.7.  $L_{disp}$  indicates disparity loss. The best results are **bold**, and the second best results are underlined. We report the results in  $AP|_{R40}$ .

not related to depth-aware feature learning in supplementary material.

### 4. YOLOStereo3D with Pseudo-Stereo Views

We apply the feature-level virtual view generation that is our best method to the stereo 3D detector YOLOStereo3D [5] for monocular 3D detection. Note that the YOLO is a general architecture for image-based detection tasks, and our method is effective with a general image-based detection architecture for detecting 3D objects from a single image.

**Preliminaries of YOLOStereo3D.** The network architecture of YOLOStereo3D [5] includes four components. **(I)** A ResNet-34 [4] with shared weights is used to extract the multi-scale features from the left-right image pair. **(II)** A multi-scale stereo matching and fusion module is used to fuse the left features and the right features. **(III)** Disparity estimation head, and **(IV)** 3D detection head.

**Implementation Details.** We only modify the component **I** and use our feature-level generation method to generate the multi-scale virtual right features to adapt YOLOStereo3D to monocular 3D detection. For training, the batch size is set to 8 and other hyper-parameters are set the same as YOLOStereo3D [5]. To show the effect of the disparity loss, we conduct two experiments with disparity loss and without disparity loss.

**Results.** As shown in Table. 3, The adaptation of YOLOStereo3D [5] to monocular 3D detection with our Pseudo-Stereo views achieves significant improvements against YOLOMono3D [5] that is the official monocular version of YOLOStereo3D [5]. Also, it achieves better performance in monocular 3D detection than other state-of-the-art monocular 3D detectors, such as Pseudo-LiDAR [8], AM3D [6], DDMP-3D [7], M3D-RPN [1] and D4LCN [2]. With the disparity loss that is originally assembled in YOLOStereo3D [5], the adaptation of YOLOStereo3D [5] to monocular 3D detection with our Pseudo-Stereo views achieves significant improvements, which lies in the depth-aware feature learning with the disparity guidance in the

| Input                  | Output       | Module Config                                                       | Channel | Size                        |
|------------------------|--------------|---------------------------------------------------------------------|---------|-----------------------------|
| $I_L, \hat{I}_R$       | <i>conv1</i> | $7 \times 7$ Conv, stride=2                                         | 64      | $H/2 \times W/2$            |
| <i>conv1</i>           | <i>conv2</i> | BasicBlock $\times 3$ , dilation=1, stride=1                        | 64      | $H/2 \times W/2$            |
| <i>conv2</i>           | <i>conv3</i> | BasicBlock $\times 4$ , dilation=1, stride=2                        | 128     | $H/4 \times W/4$            |
| <i>conv3</i>           | <i>conv4</i> | BasicBlock $\times 6$ , dilation=2, stride=1                        | 128     | $H/4 \times W/4$            |
| <i>conv4</i>           | <i>conv5</i> | BasicBlock $\times 3$ , dilation=4, stride=1                        | 128     | $H/4 \times W/4$            |
| <i>conv5</i>           | <i>spp1</i>  | AvgPool ( $64 \times 64$ ); $1 \times 1$ Conv; Upsample $64 \times$ | 32      | $H/4 \times W/4$            |
| <i>conv5</i>           | <i>spp2</i>  | AvgPool ( $32 \times 32$ ); $1 \times 1$ Conv; Upsample $32 \times$ | 32      | $H/4 \times W/4$            |
| <i>conv5</i>           | <i>spp3</i>  | AvgPool ( $16 \times 16$ ); $1 \times 1$ Conv; Upsample $16 \times$ | 32      | $H/4 \times W/4$            |
| <i>conv5</i>           | <i>spp4</i>  | AvgPool ( $8 \times 8$ ); $1 \times 1$ Conv; Upsample $8 \times$    | 32      | $H/4 \times W/4$            |
| <i>spp1-4, conv3-5</i> | <i>spp</i>   | Concat                                                              | 512     | $H/4 \times W/4$            |
| <i>conv2</i>           | <i>hres1</i> | $1 \times 1$ Conv                                                   | 64      | $H/2 \times W/2$            |
| $I_L, \hat{I}_R$       | <i>hres2</i> | $1 \times 1$ Conv                                                   | 32      | $H \times W$                |
| <i>spp</i>             | <i>up1</i>   | $3 \times 3$ Conv; Upsample $2 \times$ ; Add <i>hres1</i> ; ReLU    | 64      | $H/2 \times W/2$            |
| <i>up1</i>             | <i>up2</i>   | $3 \times 3$ Conv; Upsample $2 \times$ ; Add <i>hres2</i> ; ReLU    | 32      | $H \times W$                |
| <i>up2</i>             | $F_{L/R}$    | $3 \times 3$ Conv $\times 2$                                        | 32, 32  | $H \times W$                |
| $F_{L/R}$              | $V_{st}$     | Build stereo volume(Eqn. 3), disparity downsample=1                 | 64      | $D/4 \times H/4 \times W/4$ |

Table 4. Architecture details of stereo image feature extraction with *image-level generation*.

| Input                    | Output        | Module Config                                                       | Channel | Size                        |
|--------------------------|---------------|---------------------------------------------------------------------|---------|-----------------------------|
| $I_L, D$                 | <i>conv1</i>  | $7 \times 7$ Conv, stride=2                                         | 64      | $H/2 \times W/2$            |
| <i>conv1</i>             | <i>conv2</i>  | BasicBlock $\times 3$ , dilation=1, stride=1                        | 64      | $H/2 \times W/2$            |
| <i>conv2</i>             | <i>conv3</i>  | BasicBlock $\times 4$ , dilation=1, stride=2                        | 128     | $H/4 \times W/4$            |
| <i>conv3</i>             | <i>conv4</i>  | BasicBlock $\times 6$ , dilation=2, stride=1                        | 128     | $H/4 \times W/4$            |
| <i>conv4</i>             | <i>conv5</i>  | BasicBlock $\times 3$ , dilation=4, stride=1                        | 128     | $H/4 \times W/4$            |
| <i>conv3</i>             | <i>conv3'</i> | DDC                                                                 | 128     | $H/4 \times W/4$            |
| <i>conv4</i>             | <i>conv4'</i> | DDC                                                                 | 128     | $H/4 \times W/4$            |
| <i>conv5</i>             | <i>conv5'</i> | DDC                                                                 | 128     | $H/4 \times W/4$            |
| <i>conv5'</i>            | <i>spp1</i>   | AvgPool ( $64 \times 64$ ); $1 \times 1$ Conv; Upsample $64 \times$ | 32      | $H/4 \times W/4$            |
| <i>conv5'</i>            | <i>spp2</i>   | AvgPool ( $32 \times 32$ ); $1 \times 1$ Conv; Upsample $32 \times$ | 32      | $H/4 \times W/4$            |
| <i>conv5'</i>            | <i>spp3</i>   | AvgPool ( $16 \times 16$ ); $1 \times 1$ Conv; Upsample $16 \times$ | 32      | $H/4 \times W/4$            |
| <i>conv5'</i>            | <i>spp4</i>   | AvgPool ( $8 \times 8$ ); $1 \times 1$ Conv; Upsample $8 \times$    | 32      | $H/4 \times W/4$            |
| <i>spp1-4, conv3'-5'</i> | <i>spp</i>    | Concat                                                              | 512     | $H/4 \times W/4$            |
| <i>spp</i>               | $F_{L/R}$     | $3 \times 3$ Conv $\times 2$                                        | 32, 32  | $H/4 \times W/4$            |
| $F_{L/R}$                | $V_{st}$      | Build stereo volume(Eqn. 3), disparity downsample=4                 | 64      | $D/4 \times H/4 \times W/4$ |

Table 5. Architecture details of stereo image feature extraction with *feature-level generation*.

| Input                  | Output       | Module Config                                                       | Channel | Size                        |
|------------------------|--------------|---------------------------------------------------------------------|---------|-----------------------------|
| $I_L$                  | <i>conv1</i> | $7 \times 7$ Conv, stride=2                                         | 64      | $H/2 \times W/2$            |
| <i>conv1</i>           | <i>conv2</i> | BasicBlock $\times 3$ , dilation=1, stride=1                        | 64      | $H/2 \times W/2$            |
| <i>conv2</i>           | <i>conv3</i> | BasicBlock $\times 4$ , dilation=1, stride=2                        | 128     | $H/4 \times W/4$            |
| <i>conv3</i>           | <i>conv4</i> | BasicBlock $\times 6$ , dilation=2, stride=1                        | 128     | $H/4 \times W/4$            |
| <i>conv4</i>           | <i>conv5</i> | BasicBlock $\times 3$ , dilation=4, stride=1                        | 128     | $H/4 \times W/4$            |
| <i>conv5</i>           | <i>spp1</i>  | AvgPool ( $64 \times 64$ ); $1 \times 1$ Conv; Upsample $64 \times$ | 32      | $H/4 \times W/4$            |
| <i>conv5</i>           | <i>spp2</i>  | AvgPool ( $32 \times 32$ ); $1 \times 1$ Conv; Upsample $32 \times$ | 32      | $H/4 \times W/4$            |
| <i>conv5</i>           | <i>spp3</i>  | AvgPool ( $16 \times 16$ ); $1 \times 1$ Conv; Upsample $16 \times$ | 32      | $H/4 \times W/4$            |
| <i>conv5</i>           | <i>spp4</i>  | AvgPool ( $8 \times 8$ ); $1 \times 1$ Conv; Upsample $8 \times$    | 32      | $H/4 \times W/4$            |
| <i>spp1-4, conv3-5</i> | <i>spp</i>   | Concat                                                              | 512     | $H/4 \times W/4$            |
| <i>spp</i>             | $F_{L/R}$    | $3 \times 3$ Conv $\times 2$ ; Clone                                | 32, 32  | $H/4 \times W/4$            |
| $F_{L/R}$              | $V_{st}$     | Build stereo volume(Eqn. 3), disparity downsample=4                 | 64      | $D/4 \times H/4 \times W/4$ |

Table 6. Architecture details of stereo image feature extraction with *feature clone*.

overall loss function.

## 5. The architecture details of the proposed three methods

In the paper, we propose three novel methods to generate the virtual right view: (a) *image-level generation*, (b) *feature-level generation* and (c) *feature-clone*. We use LIGA-Stereo [3] as our base stereo 3D architecture and feed the Pseudo-Stereo views to LIGA-Stereo. We only modify the component of stereo image feature extraction in LIGA-Stereo [3] for monocular 3D detection. Table. 4 shows the architecture of stereo image feature extraction with *image-level generation*. Table. 5 shows the architecture of stereo image feature extraction with *feature-level generation*. Table. 6 the architecture of stereo image feature extraction with *feature-clone*.

## References

- [1] Garrick Brazil and Xiaoming Liu. M3d-rpn: Monocular 3d region proposal network for object detection. In *Proceedings of the IEEE International Conference on Computer Vision*, pages 9287–9296, 2019.
- [2] Mingyu Ding, Yuqi Huo, Hongwei Yi, Zhe Wang, Jianping Shi, Zhiwu Lu, and Ping Luo. Learning depth-guided convolutions for monocular 3d object detection. *arXiv preprint arXiv:1912.04799*, 2019.
- [3] Xiaoyang Guo, Shaoshuai Shi, Xiaogang Wang, and Hongsheng Li. Liga-stereo: Learning lidar geometry aware representations for stereo-based 3d detector. In *Proceedings of the IEEE/CVF International Conference on Computer Vision*, pages 3153–3163, 2021.
- [4] Kaiming He, Xiangyu Zhang, Shaoqing Ren, and Jian Sun. Deep residual learning for image recognition. In *Proceedings of the IEEE conference on computer vision and pattern recognition*, pages 770–778, 2016.
- [5] Yuxuan Liu, Lujia Wang, and Ming Liu. Yolostereo3d: A step back to 2d for efficient stereo 3d detection. *arXiv preprint arXiv:2103.09422*, 2021.
- [6] Xinzhu Ma, Zhihui Wang, Haojie Li, Pengbo Zhang, Wanli Ouyang, and Xin Fan. Accurate monocular 3d object detection via color-embedded 3d reconstruction for autonomous driving. In *Proceedings of the IEEE International Conference on Computer Vision*, pages 6851–6860, 2019.
- [7] Li Wang, Liang Du, Xiaoqing Ye, Yanwei Fu, Guodong Guo, Xiangyang Xue, Jianfeng Feng, and Li Zhang. Depth-conditioned dynamic message propagation for monocular 3d object detection. In *Proceedings of the IEEE/CVF Conference on Computer Vision and Pattern Recognition*, pages 454–463, 2021.
- [8] Yan Wang, Wei-Lun Chao, Divyansh Garg, Bharath Hariharan, Mark Campbell, and Kilian Q Weinberger. Pseudo-lidar from visual depth estimation: Bridging the gap in 3d object detection for autonomous driving. In *Proceedings of the IEEE Conference on Computer Vision and Pattern Recognition*, pages 8445–8453, 2019.
